# Supplementary material for: High-fidelity holographic beam shaping with optimal transport and phase diversity
Source: arXiv:2408.17025 ancillary file (2026-01-06)
Supplement: Supplementary file 1 [file Supplement.pdf]

# High-fidelity holographic beam shaping with optimal transport and phase diversity: supplemental document

HUNTER SWAN<sup>1,\*</sup>, ANDRII TORCHYLO<sup>1</sup>,  
MICHAEL J. VAN DE GRAAFF<sup>1</sup>, JAN RUDOLPH<sup>1,2</sup>, AND  
JASON M. HOGAN<sup>1,+</sup>

<sup>1</sup>Department of Physics, Stanford University, Stanford, California 94305, USA

<sup>2</sup>Fermi National Accelerator Laboratory, Batavia, Illinois 60510, USA

\*orswan@stanford.edu

+hogan@stanford.edu

## 1. INTRODUCTION

Sections of this supplementary document correspond to same numbered sections in the main manuscript, and provide derivations and more detailed explanations.

## 2. SETUP AND MATHEMATICAL FORMULATION

The goal of this section is to provide justification for Eqs. (1, 3, 8, 9, 12). We temporarily abandon our convention of using units of  $\sqrt{f\lambda}$  for distances. Our starting point will be the formula for propagation of light in free space under the paraxial approximation. Let  $\mathbf{u}(x, y, z)e^{2\pi i t c/\lambda}$  represent an electric field of frequency  $c/\lambda$  propagating paraxially in the  $+\hat{z}$  direction. Then the amplitude  $\mathbf{u}(x, y, z)$  at arbitrary  $z$  is related to that in the plane  $z = 0$  by

$$\begin{aligned}\mathbf{u}(x, y, z) &= \frac{i}{\lambda z} e^{2\pi i z/\lambda} e^{2\pi i(x^2+y^2)/2z\lambda} \iint_{\mathbb{R}^2} e^{2\pi i(v^2+w^2)/2z\lambda} e^{-2\pi i(xv+yw)/z\lambda} \mathbf{u}(v, w, 0) \, dv \, dw \\ &= \frac{i}{\lambda z} e^{2\pi i z/\lambda} e^{2\pi i(x^2+y^2)/2z\lambda} \mathcal{F} \left[ \mathbf{u}(v, w, 0) e^{2\pi i(v^2+w^2)/2z\lambda} \right] \left( \frac{x}{z\lambda}, \frac{y}{z\lambda} \right)\end{aligned}\quad (\text{S1})$$

See e.g. Dickey [1] Eq. (2.238) for a derivation of this formula.

A lens of focal length  $f$  centered on the  $z$ -axis affects an electric field amplitude  $\mathbf{u}$  as above by multiplying a quadratic phase  $\exp(-2\pi i(x^2 + y^2)/2f\lambda)$  (cf. Dickey [1] 2.6.3). Choosing coordinates such that the plane of the SLM in Fig. (1) corresponds to  $z = 0$ , the electric field at the plane of the camera  $\mathbf{u}(X, Y, 2f)$  is related to that at the plane of the SLM  $\mathbf{u}(x, y, 0)$  by free propagation for distance  $f$ , followed by multiplication by phase  $\exp(-2\pi i(v^2 + w^2)/2f\lambda)$  (where coordinates  $v, w$  parametrize the plane of the lens), followed by free propagation by distance  $f$ .

The combined effect of these three transformations yields

$$\begin{aligned}
\mathbf{u}(X, Y, 2f) &= - \left( \frac{e^{2\pi i f / \lambda}}{f \lambda} \right)^2 e^{2\pi i (X^2 + Y^2) / 2f \lambda} \iint_{\mathbb{R}^2} e^{2\pi i (v^2 + w^2) / 2f \lambda} e^{-2\pi i (Xv + Yw) / f \lambda} \\
&\quad \iint_{\mathbb{R}^2} e^{2\pi i (x^2 + y^2) / 2f \lambda} e^{-2\pi i (vx + wy) / f \lambda} \mathbf{u}(x, y, 0) \, dx \, dy \, dv \, dw \\
&= - \left( \frac{e^{2\pi i f / \lambda}}{f \lambda} \right)^2 e^{2\pi i (X^2 + Y^2) / 2f \lambda} \iiint_{\mathbb{R}^4} e^{2\pi i ((v-x-X)^2 + (w-y-Y)^2) / 2f \lambda} \\
&\quad e^{-2\pi i (xX + yY) / f \lambda} e^{-2\pi i (X^2 + Y^2) / 2f \lambda} \mathbf{u}(x, y, 0) \, dv \, dw \, dx \, dy \\
&= - \left( \frac{e^{2\pi i f / \lambda}}{f \lambda} \right)^2 (if \lambda) \iint_{\mathbb{R}^2} e^{-2\pi i (xX + yY) / f \lambda} \mathbf{u}(x, y, 0) \, dx \, dy \\
&= \frac{-ie^{4\pi i f / \lambda}}{f \lambda} \mathcal{F}[\mathbf{u}(x, y, 0)] \left( \frac{X}{f \lambda}, \frac{Y}{f \lambda} \right). \tag{S2}
\end{aligned}$$

Defining dimensionless coordinates  $x' = x / \sqrt{f \lambda}$ ,  $X' = X / \sqrt{f \lambda}$ , etc., and fields

$$\begin{aligned}
\mathbf{a}(x', y') &:= \mathbf{u}(x' \sqrt{f \lambda}, y' \sqrt{f \lambda}, 0), \\
\mathbf{A}(X', Y') &:= \mathbf{u}(X' \sqrt{f \lambda}, Y' \sqrt{f \lambda}, 2f),
\end{aligned}$$

Eq. (S2) becomes

$$\begin{aligned}
\mathbf{A}'(X', Y') &= -ie^{4\pi i f / \lambda} \iint_{\mathbb{R}^2} e^{-2\pi i (x' X' + y' Y')} \mathbf{a}(x', y') \, dx' \, dy' \\
&= -ie^{4\pi i f / \lambda} \mathcal{F}[\mathbf{a}(x', y')] (X', Y'),
\end{aligned}$$

which is Eq. (1) up to an overall phase, which we may ignore. We will henceforth drop the primes and work exclusively with the non-dimensionalized variables and fields.

An additional result we will need is the stationary phase approximation (SPA), which states the following. Given a function  $g : \mathbb{R}^n \rightarrow \mathbb{C}$  which decays exponentially at infinity, a function  $f : \mathbb{R}^n \rightarrow \mathbb{R}$  whose critical points are all non-degenerate (i.e. at all points  $\mathbf{x}$  such that  $\nabla f(\mathbf{x}) = 0$ , we have  $\det Hf(\mathbf{x}) \neq 0$ ), and a real scalar  $k \in \mathbb{R}$ , in the limit  $k \rightarrow \infty$  we have

$$\int_{\mathbb{R}^n} g(\mathbf{x}) e^{ikf(\mathbf{x})} \, d\mathbf{x} = \sum_{\mathbf{x}_0} \frac{g(\mathbf{x}_0) e^{ikf(\mathbf{x}_0) + \frac{i\pi}{4} \text{sgn}(Hf(\mathbf{x}_0))}}{\left(\frac{k}{2\pi}\right)^2 \sqrt{|\det Hf(\mathbf{x}_0)|}} + o(k^{-n/2}), \tag{S3}$$

where the sum is over critical points  $\mathbf{x}_0$  of  $f$ . Here  $\text{sgn}(Hf(\mathbf{x}_0))$  denotes the signature of the Hessian matrix of  $f$  at  $\mathbf{x}_0$ , i.e. the difference of the numbers of positive and negative eigenvalues.

We will apply the SPA mostly to estimating Fourier transforms of the form

$$\iint_{\mathbb{R}^2} g(\mathbf{x}) e^{2\pi i (\psi(\mathbf{x}) - \mathbf{x} \cdot \mathbf{X})} \, d\mathbf{x},$$

with  $\psi(\mathbf{x})$  a real valued function which is strictly convex or strictly concave on the support of  $g$ . Then the sum in Eq. (S3) contains at most one term, and we find

$$\iint_{\mathbb{R}^2} g(\mathbf{x}) e^{2\pi i (\psi(\mathbf{x}) - \mathbf{x} \cdot \mathbf{X})} \, d\mathbf{x} \approx \pm \frac{ig(\mathbf{x}_0) e^{2\pi i (\psi(\mathbf{x}_0) - \mathbf{x}_0 \cdot \mathbf{X})}}{\sqrt{\det H\psi(\mathbf{x}_0)}} \tag{S4}$$

where  $\mathbf{x}_0$  satisfies  $\nabla \psi(\mathbf{x}_0) = \mathbf{X}$  and the  $+$  ( $-$ ) sign corresponds to  $\psi$  convex (concave). Taking the absolute value of both sides of this equation yields Eq. (3).

### A. Phase Diversity

If  $g(\mathbf{x})$ ,  $\psi(\mathbf{x})$  represent the true input beam modulus and phase in the context of phase diversity imaging, then the electric field of the  $j$ -th diversity image is given by

$$G_j(\mathbf{X}) e^{2\pi i \Phi_j(\mathbf{X})} = \mathcal{F} \left[ g(\mathbf{x}) e^{2\pi i (\psi(\mathbf{x}) + \alpha_j x^2 / 2)} \right] (\mathbf{X}) = \iint_{\mathbb{R}} g(\mathbf{x}) e^{2\pi i (\psi(\mathbf{x}) + \alpha_j x^2 / 2 - \mathbf{x} \cdot \mathbf{X})} \tag{S5}$$

Applying Eq. (S4) yields Eqs. (8, 9), up to an irrelevant overall phase.

We next establish the relationship (12) between the electric fields of two different diversity phases  $\alpha_j, \alpha_k$ . Inverting Eq. (S5),

$$g(\mathbf{x})e^{2\pi i\psi(\mathbf{x})} = e^{-2\pi i\alpha_j x^2/2} \mathcal{F}^{-1} \left[ G_j(\mathbf{X}) e^{2\pi i\Phi_j(\mathbf{X})} \right](\mathbf{x}). \quad (\text{S6})$$

Combining Eq. (S5) (with index  $j$  replaced by  $k$  everywhere) and Eq. (S6) yields

$$\begin{aligned} G_k(\mathbf{X}) e^{2\pi i\Phi_k(\mathbf{X})} &= \mathcal{F} \left[ e^{-2\pi i\Delta\alpha x^2/2} \mathcal{F}^{-1} \left[ G_j(\mathbf{Y}) e^{2\pi i\Phi_j(\mathbf{Y})} \right](\mathbf{x}) \right](\mathbf{X}) \\ &= \iint_{\mathbb{R}^2} \iint_{\mathbb{R}^2} e^{2\pi i(\Phi_j(\mathbf{Y}) - \Delta\alpha x^2/2 + \mathbf{x} \cdot (\mathbf{Y} - \mathbf{X}))} G_j(\mathbf{Y}) d\mathbf{Y} d\mathbf{x} \\ &= \iint_{\mathbb{R}^2} \left( \iint_{\mathbb{R}^2} e^{2\pi i(-\Delta\alpha(\mathbf{x} - (\mathbf{Y} - \mathbf{X})/\Delta\alpha)^2/2)} d\mathbf{x} \right) e^{2\pi i(\Phi_j(\mathbf{Y}) + (\mathbf{Y} - \mathbf{X})^2/2\Delta\alpha)} G_j(\mathbf{Y}) d\mathbf{Y} \\ &= \left( \frac{1}{i\Delta\alpha} \right) e^{2\pi iX^2/2\Delta\alpha} \iint_{\mathbb{R}^2} e^{2\pi i(\Phi_j(\mathbf{Y}) + Y^2/2\Delta\alpha - \mathbf{Y} \cdot \mathbf{X}/\Delta\alpha)} G_j(\mathbf{Y}) d\mathbf{Y} \\ &= \frac{1}{i\Delta\alpha} e^{2\pi iX^2/2\Delta\alpha} \mathcal{F} \left[ e^{2\pi i(\Phi_j(\mathbf{Y}) + Y^2/2\Delta\alpha)} G_j(\mathbf{Y}) \right] \left( \frac{\mathbf{X}}{\Delta\alpha} \right), \end{aligned} \quad (\text{S7})$$

which is Eq. (12). (Here as before  $\Delta\alpha := \alpha_j - \alpha_k$ .) We note that the right hand side of Eq. (S7) is closely related to a fractional Fourier transform of angle  $\cot^{-1}(1/\Delta\alpha)$ .

#### A.1. Linear phase offsets

With current technology, all real SLMs exhibit a “zero order spot”, which manifests as a bright spot where the camera plane intersects the optical axis. This spot is due to input beam light which is not phase modulated by the SLM, such as the light incident on the regions in between SLM pixels. In current devices, around 10% of the input beam power is typically diffracted into the zero order spot.

In order to avoid corruption of the output image due to interference with the zero order spot, it is convenient to add an additional linear component to all SLM phases, which provides a uniform shift of the output beam. In the context of phase diversity imaging, this means that the actual diversity phases we use have the form

$$\alpha_j x^2/2 + \boldsymbol{\beta} \cdot \mathbf{x}$$

for some common vector  $\boldsymbol{\beta} \in \mathbb{R}^2$ . This has the effect of translating all output beams by  $\boldsymbol{\beta}$ . With this modification, Eq. (8) is unchanged in form, and Eq. (9) acquires a third term, giving

$$G_j(\mathbf{X}) \approx \frac{g(\mathbf{x})}{\sqrt{\alpha_j^2 + \alpha_j \text{Tr} H\psi(\mathbf{x}) + \det H\psi(\mathbf{x})}} \quad (\text{S8})$$

$$\Phi_j(\mathbf{X}) \approx \alpha_j x^2/2 + \boldsymbol{\beta} \cdot \mathbf{x} - \mathbf{x} \cdot \mathbf{X}, \quad (\text{S9})$$

with  $\mathbf{x}$  now satisfying  $\nabla\psi(\mathbf{x}) + \alpha_j \mathbf{x} + \boldsymbol{\beta} = \mathbf{X}$ . Eqs. (10) and (11) become

$$g(\mathbf{x}) \approx |\alpha_j| G_j(\alpha_j \mathbf{x} + \boldsymbol{\beta}) \quad (\text{S10})$$

and

$$g(\mathbf{x}) \approx \left| \mathcal{F}^{-1} \left[ G_j(\mathbf{X}) \exp \left( -2\pi i(\mathbf{X} - \boldsymbol{\beta})^2/(2\alpha_j) \right) \right] \right|, \quad (\text{S11})$$

respectively. Eqs. (12, 13) are unchanged.

#### B. Discretization and Fourier duality

For computational solution of the phase generation problem, we discretize the beam moduli and phase functions of Problem (1) onto rectangular grids:  $(x_0 + j\Delta x, y_0 + k\Delta y)$ ,  $j = 0, \dots, n_x - 1$ ,  $k = 0, \dots, n_y - 1$ , in the SLM plane; and  $(X_0 + J\Delta X, Y_0 + K\Delta Y)$ ,  $J = 0, \dots, N_X - 1$ ,  $K = 0, \dots, N_Y - 1$  in the camera plane. It is often convenient for these grids to be dual to each other in the Fourier sense, for in this case the discrete Fourier transform (DFT) of a function sampled on the grid provides a very good approximation to the (continuous) Fourier transform of the function [2],

modulo a linear phase which depends on the grid offsets  $x_0, y_0$ . Specifically, Fourier duality requires that the number and size of steps in the various grid directions satisfy

$$\begin{aligned} n_x &= N_X = 1/\Delta x \Delta X, \\ n_y &= N_Y = 1/\Delta y \Delta Y. \end{aligned}$$

For any integers  $n_x, n_y$ , there is a unique grid  $\mathcal{L}_{n_x, n_y}$  of size  $n_x \times n_y$  which is self-dual and satisfies  $x_0 + \lfloor n_x/2 \rfloor \Delta x = y_0 + \lfloor n_y/2 \rfloor \Delta y = 0$ , where the latter condition indicates that the grid is centered about 0. We refer to this grid as the “natural lattice” of size  $n$ . Explicitly, in this case we have  $\Delta x = 1/\sqrt{n_x}$ ,  $\Delta y = 1/\sqrt{n_y}$ ,  $x_0 = -\lfloor n_x/2 \rfloor / \sqrt{n_x}$ , and  $y_0 = -\lfloor n_y/2 \rfloor / \sqrt{n_y}$ .

At any point in this work where we perform a Fourier transform on simulation data (in particular, in the GS, MRAF, and phase diversity IFT algorithms), it suffices to assume that all fields are defined on a natural lattice, or more generally any dual pair of grids. Note however that duality is not required for grids in OT based algorithms. This latter fact is very useful, as it allows us to freely crop or downsample inputs to the OT algorithms, without having to ensure duality to any other grids.

### 3. ALGORITHMS FOR PHASE GENERATION

#### A. Algorithm details

In this section we show more explicitly the steps presented in Sec. (3) for solving the phase generation problem with optimal transport. The array flattening and reshaping of steps 1 and 3 is discussed below in (A.1). The form of the cost matrix is also discussed in (A.1). The OT solver of step 2 is discussed in (A.2). The first moment computation of step 4 for determining the transport map  $\gamma$  from the transport plan  $\Gamma$  is discussed in (A.3). The integration of step 5 is discussed in (A.4).

The data for the phase generation problem consist of input and output grids  $(x_0 + j\Delta x, y_0 + k\Delta y)$ ,  $(X_0 + J\Delta X, Y_0 + K\Delta Y)$  and input and output intensity arrays  $g_{jk}^2, G_{JK}^2$ , with indices  $j = 0, \dots, n_x - 1, k = 0, \dots, n_y - 1, J = 0, \dots, N_X - 1, K = 0, \dots, N_Y - 1$ . The output of our algorithm will be a phase array  $\phi_{jk}$ . For notational simplicity, we will assume square arrays and set  $n := n_x = n_y = N_X = N_Y$ . We let  $x_j$  denote  $x_0 + j\Delta x$ , and similarly for other coordinates.

#### A.1. Flattening and unflattening

The two-dimensional arrays  $g_{jk}^2, G_{JK}^2$  representing the input and target beam intensities must be flattened to interface with OT solvers. Any method for flattening may be used, but care must be taken to ensure that the cost matrix is constructed in a manner consistent with the flattening operation. We will describe the structure of the cost matrix in the case of Julia-style, row-first array flattening. In this case, matrix  $g_{jk}^2, j, k = 0, \dots, n - 1$ , is flattened to a vector  $\mu_j = g_{(j\%n)(\lfloor j/n \rfloor)}^2$ ,  $i = 0, \dots, n^2 - 1$ , where  $i\%n$  denotes the remainder of  $i$  by  $n$ . To reshape a vector like  $\mu_j$  back to a matrix like  $g_{jk}^2$ , we have the formula  $g_{jk}^2 = \mu_{j+nk}$ .

The input grid point corresponding to flattened vector entry  $j$  is  $(x_{j\%n}, y_{\lfloor j/n \rfloor})$ , and similarly for output grid points. Thus the cost matrix entry  $c_{jK}$ , which represents the squared distance between flattened input grid point  $j$  and flattened output grid point  $K$ , is

$$c_{jK} = \left( x_{(j\%n)} - X_{(K\%n)} \right)^2 + \left( y_{\lfloor j/n \rfloor} - Y_{\lfloor K/n \rfloor} \right)^2, \quad (\text{S12})$$

which is Eq. (17). This cost matrix is visualized in Fig. (S1). As discussed below in (A.2), we sometimes compute the cost matrix using a different pair of grids than  $(x_j, y_k), (X_J, Y_K)$ .

The cost matrix  $c_{jK}$  can be reshaped to a four dimensional array  $c'_{jklM}$  which represents the squared distance between points  $(x_j, y_k)$  in the input plane and  $(X_L, Y_M)$  in the output plane. The formula for such reshaping is  $c'_{jklM} = c_{(j+nk)(L+nM)}$ . Similarly, the transport plan returned by the OT solver comes as a matrix  $\Gamma'_{jK}$  which we reshape to a four dimensional array  $\Gamma'_{jklM} = \Gamma'_{(j+nk)(L+nM)}$ .

#### A.2. OT solver optimization

Various OT solvers are available through the Julia package OptimalTransport.jl[3], but the “sinkhorn” function has the best computational complexity. This function generates an approximate solution to an OT problem by incorporating an entropic regularization. The regularization is

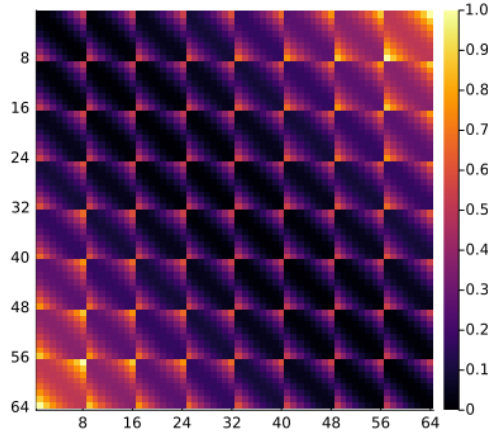

**Fig. S1.** Visualization of the cost matrix for the OT algorithm. Color indicates magnitude of a matrix element, normalized such that the maximum value is 1. For visual clarity the cost matrix shown is that of a 2-dimensional grid with 8 points on each side, which is much smaller than the grids used in practice.

parametrized by a hyperparameter  $\epsilon$ , and one recovers an exact solution to the optimal transport problem in the limit  $\epsilon \rightarrow 0$ . We have found that a value  $\epsilon = 0.001$  works well for essentially all of our use cases.

The solution to our OT problem is nominally invariant under translations and rescalings of the input grid and output grid (and in particular, either grid may be translated or rescaled independently of the other). However, in practice the performance of a computational OT solver will suffer if the numerical values of cost matrix elements are very large, or if the input and output grids have wildly different scales. We thus find it helpful to modify the input and output grids and the resulting cost matrix in three ways. Firstly, we replace the input and output grids with the same-sized natural lattices. Secondly, we scale the points of the output lattice so that the largest coordinates have the same magnitude as the largest coordinates of the input lattice. Lastly, after computing the cost matrix, we normalize it to have largest entry equal to 1. As a concrete one-dimensional example, suppose the input and output grids are  $0, 1, \dots, 15$  and  $0, 1, \dots, 63$ , respectively. The corresponding natural lattices are  $-2, -2.25, \dots, 1.75$  and  $-4, -3.875, \dots, 3.875$ . The second grid is then rescaled to  $-2, -1.9375, \dots, 1.9375$ . Finally, the cost matrix between these two grids is normalized by dividing by the largest squared distance between points in the modified input and output grid, namely  $(1.9375 - (-2))^2$ .

### A.3. Moment computation for transport map

Given the four dimensional array  $\Gamma_{jkLM}$  as in Sec. (A.1), we next wish to compute the transport map  $\gamma_{jk,w}$ . Provided  $g_{jk}^2 = \sum_{LM} \Gamma_{jkLM}$  is non-zero, Eq. (15) becomes in the discrete setting

$$\gamma_{jk,x} = \frac{1}{g_{jk}^2} \sum_{LM} X_L \Gamma_{jkLM} \quad (\text{S13})$$

$$\gamma_{jk,y} = \frac{1}{g_{jk}^2} \sum_{LM} Y_M \Gamma_{jkLM}. \quad (\text{S14})$$

In the common scenario where the support of  $g_{jk}^2$  is a convex subset of the input plane,  $\gamma_{jk,w}$  may be defined arbitrarily at any points where  $g_{jk}^2 = 0$ , since the phase values outside of the support of  $g_{jk}^2$  do not affect the output beam shape. There could potentially be problems in defining  $\gamma_{jk,w}$  consistently if the input beam were ring shaped, with an open region of zero intensity enclosed by the support of  $g_{jk}^2$ . We have not investigated this case, but if it were found to be troublesome we expect it could be remedied by adding a small non-zero value to  $g_{jk}^2$  in its interior null regions.

#### A.4. Phase gradient integration

We compute the phase  $\phi_{jk}$  from the OT map  $\gamma_{jk,w}$  by first picking a reference point indexed by  $(j_0, k_0)$  in the input grid and integrating via the trapezoid rule, giving

$$\phi_{jk} = \left( \sum_{i=0}^j \gamma_{ik_0,x} - \sum_{i=0}^{j_0} \gamma_{ik_0,x} - \gamma_{jk_0,x}/2 \right) \Delta x + \left( \sum_{i=0}^k \gamma_{ji,y} - \sum_{i=0}^{k_0} \gamma_{ji,y} - \gamma_{jk,y}/2 \right) \Delta y. \quad (\text{S15})$$

The final term in each bracketed expression is a boundary term due to use of the trapezoid rule. Higher order quadrature rules may also be used, leading to more complicated boundary terms[4].

Since the OT map  $\gamma_{jk,w}$  represents a discretization of a gradient, if it were untarnished by numerical errors, integrating along any path would yield the same result  $\phi_{jk}$ . In practice there is some path dependence (e.g. summing row first vs. column first yields slightly different results). A potentially more accurate method for recovering  $\phi_{jk}$  from  $\gamma_{jk,w}$  would be to use Helmholtz-Hodge decomposition, which resolves  $\gamma_{jk,w}$  into harmonic, curl-free, and solenoidal components. The curl-free part may provide a better estimate for the true value of  $\phi_{jk}$ . We have not pursued this avenue, since we only need the OT solution to be sufficiently accurate as to yield a good starting guess for an iterative algorithm such as GS or MRAF. The above quadrature method successfully accomplishes this.

#### B. Performance

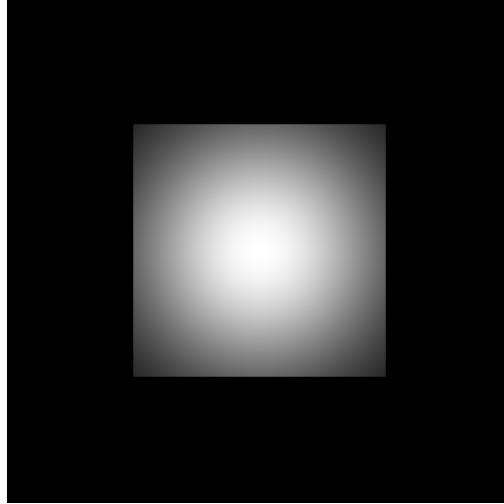

**Fig. S2.** Input beam intensity for generating Table (1).

Our main aim in this subsection is to discuss the methods involved in making Table (1). In making this comparison, we have tried to carefully reproduce input and target output beam characteristics defined in [5]. We summarize these characteristics below in our own nomenclature.

The SLM grid is taken to have size  $768 \times 768$  with step size 1, embedded in the center of a larger computational grid of size  $1536 \times 1536$ . The input beam is taken to be a centered Gaussian with modulus  $g(\mathbf{x}) \propto \exp(-x^2/\omega^2)$ , with  $\omega = 565$ , in the central  $768 \times 768$  SLM region, and 0 outside of this region. This models the physical scenario of a large Gaussian clipped by the aperture of an SLM. The intensity of the input beam is shown in Fig. (S2).

The target output beams are shown in Fig. (S3). All units in the following descriptions are pixels. The first target is a Gaussian ring of radius 53, thickness 14, and height 1 superposed on two Gaussians of radius 7 and height 2 at the north and south pole of the ring. The second is a three-pointed star with outer radius 40 and inner radius 10, convolved with a Gaussian of radius 5. The third is a square of side length 116 convolved with a  $9 \times 9$  averaging filter. The fourth is a representation of an “atomtronic OR gate” with an overall height of 325 pixels, with detailed dimensions available in the source code[6]. The fifth is a Gaussian ring of radius 53, thickness 14, with two Gaussian tails of length  $\approx 40$  and thickness 14, and a band of height 10 in the middle of the ring where the intensity is reduced by a factor of 2. The sixth is the pointwise max of a Gaussian wire of length 264 and thickness 7 and a pair of Gaussians of radius 17.6

located at the ends of the wire. (We remark that we believe there to be a few inconsistencies in the descriptions of target geometries in [5], and some of the numbers we state above differ from theirs—e.g. the outer radius of the second target. We have attempted to give our best estimate of the true parameters for a fair comparison between our work and theirs.)

The targets are embedded in a lattice dual to the  $1536 \times 1536$  input grid. Explicitly, the dual lattice has the form  $(-0.5 + j/1536, -0.5 + k/1536)$ ,  $j, k = 0, \dots, 1535$ . Targets 1, 4, 5, and 6 are centered on this output grid, while target 2 is shifted  $45^\circ$  up and left by 37 pixels, and target 3 is shifted left by 63 pixels.

The OT solutions for the phase generation problems so posed are shown in Fig. (S4). In computing the OT solution, we crop the target output beam to a  $200 \times 200$  window for targets 1, 2, 3, and 5, and to a  $400 \times 400$  window for targets 4 and 6. We then downsample to  $100 \times 100$  pixels. We crop the input beam to the central  $800 \times 800$  pixel region and downsample to  $100 \times 100$  pixels.

For MRAF iterations we must define a signal region where the algorithm attempts to optimize the output beam intensity. We use the same signal regions as [5]. For the first target, this is an annular region with inner radius 25 and outer radius 81. For the second, it is a disk of radius 40. For the third, it is a square of side length 151. For the fourth and fifth it is the locus of points which are within distance 10 of a pixel with intensity at least 10% of the maximum intensity. For the sixth, it consists of two disks of radius 53 centered on the end Gaussians, together with a connecting strip of width 25. These same regions are used for the computation of the efficiency statistic  $\eta$  for all output beams (i.e. those generated by OT, GS, and MRAF).

The output beams after tuning the OT solutions with 1000 MRAF iterations are shown in Fig. (S5). We tuned the MRAF mixing parameter  $m$  by hand for each target, and the values used were 0.460, 0.455, 0.455, 0.421, 0.480, 0.480, respectively.

We mention that it is possible to make the signal region for the MRAF algorithm the entire  $200 \times 200$  or  $400 \times 400$  bounding box displayed in Fig. (S3) while maintaining good accuracy and efficiency. The results of doing so are shown in Fig. (S6), using the same mixing parameters and number of iterations as for Fig. (S5). There is no comparison for this in [5].

As a final step before computing RMS error and efficiency for comparison to [5], we round the phase at each pixel to 256 values, evenly spaced from  $-\pi$  to  $\pi$ . This was a non-ideal effect modelled by the same reference. We find this changes the accuracy and efficiency of the output beam very little (typically at the hundredth of a percent level).

In defining the RMS error via Eq. (18), we defined the “measure region”  $U$  as the locus of pixels where the target intensity attains at least fraction  $1/10$  of its maximum value. In [5] this definition was used for four of the six targets, but for target 1 it was defined as an annulus of inner radius 44 and outer radius 62, and for target 3 it was defined as a square of side length 114. If we use these regions to compute the error metric for our MRAF+OT solutions (Fig. (S5)), the RMS error

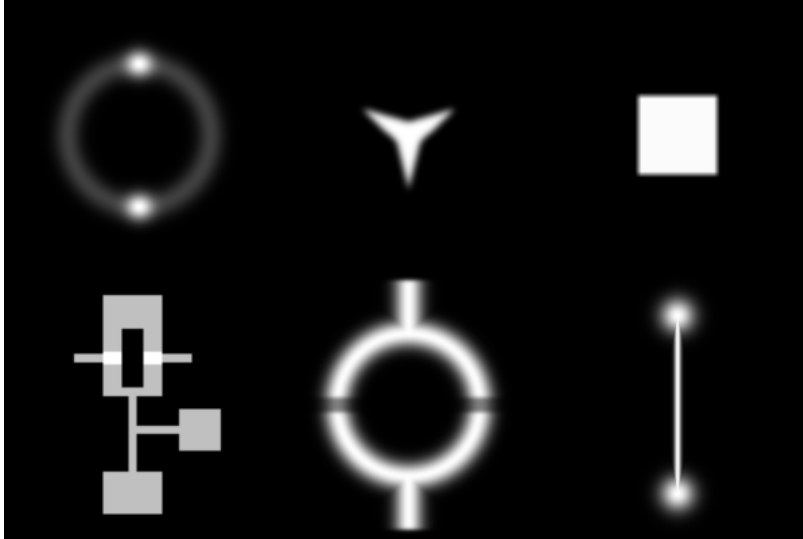

**Fig. S3.** Target output beams for generating Table (1). The field of view is  $200 \times 200$  pixels for targets 1, 2, 3, and 5, and  $400 \times 400$  for targets 4 and 6.

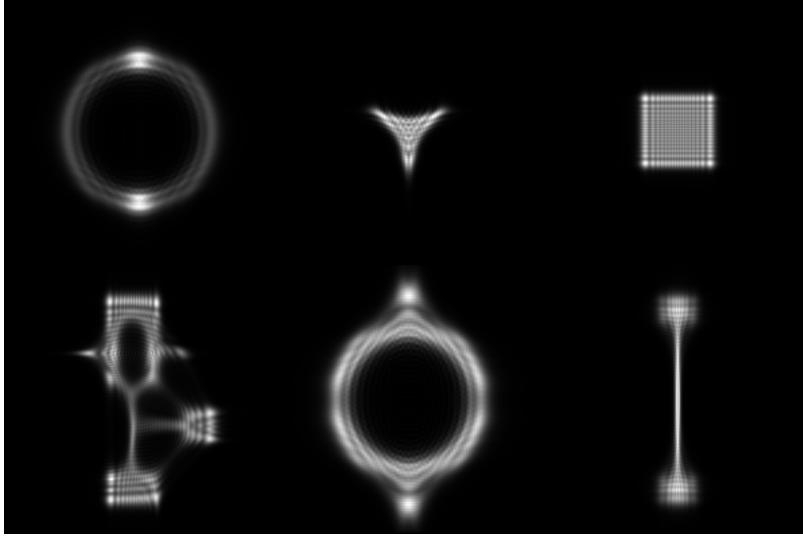

**Fig. S4.** OT solutions for each of the targets of Fig. (S3). The RMS errors and efficiencies are respectively 8.8% and 98.9%, 18.7% and 98.7%, 23.7% and 99.3%, 41.2% and 97.2%, 15.9% and 98.9%, and 11.4% and 98.8%.

becomes 0.16% and 0.44% for targets 1 and 3, respectively, instead of 0.17% and 0.78%. Thus our stated numbers in the main text are slightly more conservative.

### C. Memory requirements and multiscale methods

The size of the cost matrix and transport plan for the OT phase generation algorithm is equal to the product of the number of pixels in the input and output domains. For megapixel images, this would require 8 terabytes of memory for each, which is untenable. For large images in practice we solve this issue by cropping or downsampling the images to dimensions of roughly  $150 \times 150$  or smaller, which requires at most a few gigabytes of memory.

An alternative method for dealing with this situation, which we have not implemented, would be to run an OT solver multiple times with progressively finer resolution and to store the cost matrix and transport plan in sparse matrices. A low resolution OT solution would allow one to

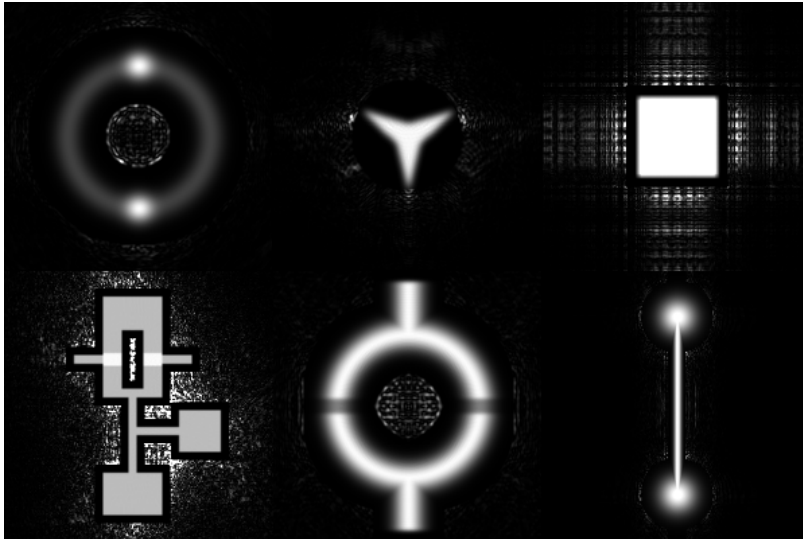

**Fig. S5.** MRAF+OT solutions for each of the targets of Fig. (S3). RMS errors and efficiencies are those of Table (1).

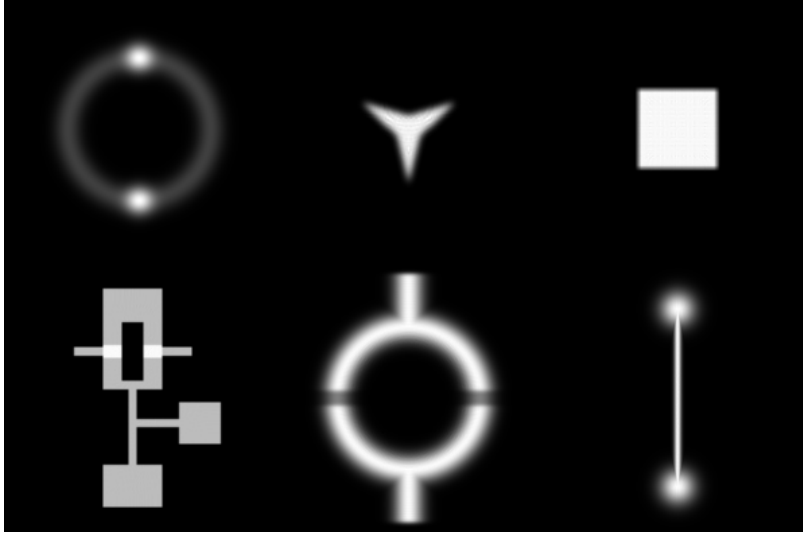

**Fig. S6.** MRAF+OT solutions for each of the targets of Fig. (S3) with signal region the full field of view. The RMS errors and efficiencies are respectively 0.14% and 72%, 1.5% and 69%, 0.95% and 70%, 0.55% and 53%, 0.40% and 85%, and 0.50% and 85%.

determine for which pairs of points  $(\mathbf{x}, \mathbf{X})$  in the input and output domains is  $\Gamma(\mathbf{x}, \mathbf{X})$  appreciable. Then when solving the problem at higher resolution, the cost matrix and transport plan would only need to be computed in the vicinity of such pairs of points. At all other points, the cost matrix would be set to  $\infty$  and the transport plan to 0.

In the Sinkhorn-Gibbs algorithm for solving optimal transport problems (which is the basis for the “sinkhorn” method of OptimalTransport.jl), the cost matrix  $c_{jK}$  only enters by way of the “Gibbs kernel”  $K_{jK} = \exp(-c_{jK}/\epsilon)$ , where  $\epsilon$  is the regularization parameter[3]. Thus in the multiscale method just described, points of infinite cost  $c_{jK} = \infty$  would translate to points where  $K_{jK} = 0$ . Since sparse matrices typically take unstored values to be zero, it is easier to work with  $K_{jK}$  directly rather than the cost matrix  $c_{jK}$  in this context.

## 4. PHASE DIVERSITY ALGORITHMS

### A. Phase retrieval theory of phase diversity imaging

In this subsection we show how the iterative Fourier transform algorithm of Section (4.A) follows naturally from general principles of phase retrieval theory. We do not assume a familiarity with phase retrieval theory, so we first review the main concepts thereof. Since we will need to index the diversity phases, images, and related objects, for the rest of this section we will drop component subscripts from all vectors to avoid confusion; all subsequent subscripts will index diversity images and related data. Absolute value signs will denote component-wise absolute value.

The basic problem of abstract phase retrieval[7] is to find a point in the intersection of two sets  $B, C \subset \mathbb{R}^n$ , making use of only the projection operators  $P_B : \mathbb{R}^n \rightarrow B$  and  $P_C : \mathbb{R}^n \rightarrow C$ , which send a point  $x \in \mathbb{R}^n$  to the nearest point of the corresponding set  $B, C$ . The GS algorithm repeatedly applies  $P_B \circ P_C$  until convergence. More sophisticated phase retrieval algorithms such as “hybrid input-output” [8] and “difference map” [9] methods use other linear combinations of compositions of the projection operators to achieve better performance on certain problems.

In the specific case of the phase generation problem for images of  $m$  pixels, the ambient space is that of all complex beam amplitudes sampled at  $m$  points, represented by a flattened vector in  $\mathbb{C}^m \cong \mathbb{R}^{2m}$  (c.f. (A.1)). The set  $B$  corresponds to those beam amplitudes  $a \in \mathbb{C}^m$  whose intensity  $|a|^2$  matches the measured input beam intensity  $g^2$ . For non-zero  $a$ , the projection  $P_B$  sends  $a \mapsto \frac{ga}{|a|}$ , which has the phase of  $a$  and the modulus of  $g$ . The set  $C$  corresponds to those beam amplitudes  $a$  whose Fourier transform (sampled on a dual grid, c.f. (B), and flattened)  $\mathcal{F}[a] = A$  has intensity  $|A|^2$  matching the desired output beam intensity  $G^2$ . The projection  $P_C$  sends  $a \mapsto \mathcal{F}^{-1} \left[ \frac{GA}{|A|} \right] = \mathcal{F}^{-1} \left[ \frac{G|\mathcal{F}[a]|}{|\mathcal{F}[a]|} \right]$ .

The phase diversity beam estimation problem differs in an important way from the phase generation problem: the latter has two constraint sets, whereas the former has one for each diversity image, of which there may be arbitrarily many. This has two consequences. Firstly, we must modify the usual phase retrieval framework to handle more than two constraints. Secondly, while phase generation is typically critically constrained, phase diversity beam estimation is overconstrained when more than two images are used. This leads to much stronger convergence of IFT algorithms for beam estimation than for phase generation.

A method for generalizing phase retrieval algorithms to more than two constraint sets has been provided in [10]. Given constraint sets  $B_j \subset \mathbb{R}^n$ ,  $j = 1, \dots, q$ , and associated projections  $P_j : \mathbb{R}^n \rightarrow B_j$ , we form the product constraint set  $C := B_1 \times \dots \times B_q \subset \mathbb{R}^{nq}$  and the diagonal constraint set  $D := \{(x, x, \dots, x) \in \mathbb{R}^{nq} : x \in \mathbb{R}^n\}$ . The projection associated to  $C$  is  $P_C := P_1 \times \dots \times P_q$ , and that associated to  $D$  is the averaging operator

$$P_D : (x_1, \dots, x_q) \mapsto \left( \frac{1}{q} \sum_j x_j, \dots, \frac{1}{q} \sum_j x_j \right).$$

A point in both  $C$  and  $D$  is of the form  $(x, x, \dots, x)$  with  $x \in B_j$  for all  $j = 1, \dots, q$ , which means that  $x$  is a solution to the problem of finding a point in the intersection of all  $B_j$ ,  $j = 1, \dots, q$ . We have thus reduced the problem of finding a point in the intersection of many sets  $B_j$  to that of finding a point in the intersection of the two larger sets  $C$  and  $D$ .

The ambient space for the beam estimation problem can be taken to be the set of all complex beam amplitudes sampled at  $m$  points,  $\mathbb{C}^m$ . Given a diversity phase  $\exp(2\pi i \alpha_j x^2/2)$  and a corresponding measured diversity image  $G_j^2$ , the associated constraint set is the collection of complex beam amplitudes  $a$  such that the intensity of the Fourier transform  $|\mathcal{F}[a \exp(2\pi i \alpha_j x^2/2)]|^2$  matches the measured diversity image intensity  $G_j^2$ . The corresponding projection operator is

$$P_j : a \mapsto \exp(-2\pi i \alpha_j x^2/2) \times \mathcal{F}^{-1} \left[ \frac{G_j \mathcal{F} \left[ a \exp \left( 2\pi i \alpha_j x^2/2 \right) \right]}{\left| \mathcal{F} \left[ a \exp \left( 2\pi i \alpha_j x^2/2 \right) \right] \right|} \right], \quad (\text{S16})$$

which is (20). We have one such projection operator for each diversity image.

We are now in a position to give the analog of the Gerchberg-Saxton algorithm for phase diversity beam estimation. Given  $q$  diversity phases  $\exp(2\pi i \alpha_j x^2/2)$  and corresponding output beam moduli  $G_j$ ,  $j = 1, \dots, q$ , we let  $P_j$  denote the associated projection operator as in Eq. (S16). Then to compute an estimate of the input beam generating the measured output beam moduli, we begin with any initial guess  $a \in \mathbb{C}^m$  for the solution and repeatedly update it via  $a \leftarrow \frac{1}{N} \sum_j P_j a$ , terminating either after a fixed number of iterations or when the error metric given in Problem (2) stagnates.

## B. One-shot beam estimation from stationary phase approximation

Our aim in this section is to understand how the value of  $\alpha_j$  controls the accuracy of the one-shot beam estimate. The diversity modulus  $G_j$  is given by

$$G_j(\mathbf{X}) = \int g(x) e^{2\pi i (\psi(x) - \mathbf{x} \cdot \mathbf{X})} e^{2\pi i \alpha_j x^2/2} d\mathbf{x}, \quad (\text{S17})$$

so SPA (S3) gives

$$G_j(\mathbf{X}) = i\alpha_j^{-1} g(\mathbf{x}_0) e^{2\pi i (\psi(\mathbf{x}_0) - \mathbf{x}_0 \cdot \mathbf{X} + \alpha_j x_0^2/2)} + o(\alpha_j^{-1}), \quad (\text{S18})$$

where as usual  $\mathbf{x}_0$  satisfies  $\nabla \psi(\mathbf{x}_0) + \alpha \mathbf{x}_0 = \mathbf{X}$ . Thus we see that the accuracy of SPA in this case is directly controlled by  $\alpha_j$ .

## C. Two-shot beam estimation from optimal transport

The steps to compute a two-shot OT beam estimate are almost identical to the steps of Sec. (3), with the following modifications:

- The problem data now consists of diversity image arrays  $G_{j,LM}^2$ ,  $G_{k,LM}^2$  defined on grids  $(X_{j,L}, Y_{j,M})$ ,  $(X_{k,L}, Y_{k,M})$ , and diversity phase coefficients  $\alpha_j$ ,  $\alpha_k$ . The output is a complex array  $a_{pq}$  defined on a grid dual to  $(X_{j,L}, Y_{j,M})$ , representing the complex input beam amplitude.
- After finding the OT map  $\gamma_{JK,W}$  for the OT problem defined by the distributions  $G_{j,LM}^2$ ,  $G_{k,LM}^2$ , the phase  $\Phi_{j,LM}$  associated to diversity modulus  $G_{j,LM}^2$  is computed via

$$\begin{aligned} \Phi_{j,LM} = & \left( \sum_{p=0}^L \gamma_{PM_0,X} - \sum_{p=0}^{L_0} \gamma_{PM_0,X} - \gamma_{LM_0,X}/2 \right) \Delta X \\ & + \left( \sum_{p=0}^M \gamma_{LP,Y} - \sum_{p=0}^{M_0} \gamma_{LP,Y} - \gamma_{LM,Y}/2 \right) \Delta Y - (X_{j,L}^2 + Y_{j,M}^2) / (2\Delta\alpha), \end{aligned} \quad (\text{S19})$$

which is the analog of Eq. (S15) for phase generation.

- With  $\Phi_{j,LM}$  in hand, the beam estimate  $a_{pq}$  is given by

$$a_{pq} = \mathcal{F}^{-1} \left[ G_{j,LM} \exp \left( 2\pi i \Phi_{j,LM} \right) \right]_{pq} \exp \left( -2\pi i \alpha_j (x_p^2 + y_q^2) / 2 \right). \quad (\text{S20})$$

Just as the accuracy of the one-shot estimate is controlled by the diversity phase coefficient  $\alpha_j$  used, the accuracy of two-shot estimation is controlled by the values  $\alpha_k$  and  $\alpha_j$ . However, understanding the effect of these parameters on the error  $\delta$  is not as easy as in the one-shot case, as Eq. (S7) has a more complicated dependence on  $\alpha_j$ ,  $\alpha_k$  than does Eq. (S17) on  $\alpha_j$ . We have investigated the variation of  $\delta$  with  $\alpha_j$ ,  $\alpha_k$  empirically, and as shown in Fig. (S7) we find the best results are obtained when one of these coefficients is moderately small and the other large.

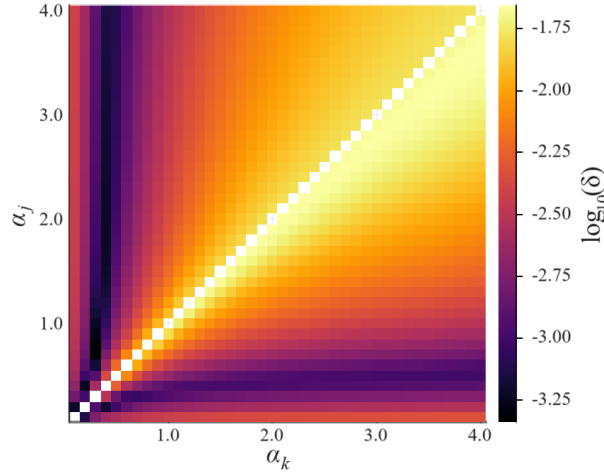

**Fig. S7.** Error  $\delta$  of an OT beam estimate for  $\alpha_j$  and  $\alpha_k$  ranging from 0.1 to 4.0. Darker regions indicate more optimal performance (i.e. smaller  $\delta$ ).

#### D. Generation of random beams

To construct the input beam for testing our beam estimation algorithms (shown in Fig. (4)), we used a sum of Hermite-Gaussian modes with random amplitudes generated as follows. The amplitude of the  $(0,0)$  mode was normalized to 1. For all other modes  $(l,m)$  with  $l, m \leq 20$ , the amplitude was given by

$$\frac{\omega_r + i\omega_i}{4(l^2 + m^2)},$$

with  $i$  the imaginary unit and  $\omega_r, \omega_i$  random variables drawn from the standard normal distribution.

## REFERENCES

1. F. M. Dickey, *Laser beam shaping: theory and techniques* (CRC press, 2018).
2. C. L. Epstein, "How well does the finite Fourier transform approximate the Fourier transform?" *Commun. on Pure Appl. Math.* **58**, 1421–1435 (2005).
3. T. Matsumoto, D. Widmann, D. Barreira, and S. Zhang, "Optimaltransport.jl," <https://github.com/JuliaOptimalTransport/OptimalTransport.jl>, commit: 9da044c (2022).
4. W. H. Press, S. A. Teukolsky, W. T. Vetterling, and B. P. Flannery, *Numerical Recipes 3rd Edition: The Art of Scientific Computing* (Cambridge University Press, USA, 2007), 3rd ed.
5. M. Pasienski and B. DeMarco, "A high-accuracy algorithm for designing arbitrary holographic atom traps," *Opt. Express* **16**, 2176–2190 (2008).
6. H. Swan, M. Van de Graaff, and A. Torchylo, "SLMTools," <https://github.com/hoganphysics/SLMTools>, commit: d7db9fd (2024).
7. V. Elser, I. Rankenburg, and P. Thibault, "Searching with iterated maps," *Proc. National Acad. Sci.* **104**, 418–423 (2007).
8. J. R. Fienup, "Phase retrieval algorithms: a comparison," *Appl. Opt.* **21**, 2758–2769 (1982).
9. V. Elser, "Phase retrieval by iterated projections," *J. Opt. Soc. Am. A* **20**, 40–55 (2003).
10. S. Gravel and V. Elser, "Divide and concur: A general approach to constraint satisfaction," *Phys. Rev. E* **78**, 036706 (2008).
